# Supplementary material for: To regulate or not: a social dynamics analysis of the race for AI supremacy
Source: arXiv:1907.12393 source file (2020-01-16)
Supplement: Supplementary file 1 [file SI.pdf]

# Supporting Information:

# To regulate or not: a social dynamics analysis of the race for AI supremacy

The Anh Han[1,*], Luís Moniz Pereira [2], Francisco C. Santos[3,4], Tom Lenaerts[4,5]

January 16, 2020

[1] School of Computing and Digital Technologies, Teesside University, Middlesbrough, UK TS1 3BA

[2] NOVA Laboratory for Computer Science and Informatics (NOVA LINCS), Universidade Nova de Lisboa, 2829-516 Caparica, Portugal

[3]INESC-ID and Instituto Superior Tecnico, Universidade de Lisboa

[4] Machine Learning Group, Université Libre de Bruxelles, Boulevard du Triomphe CP212, Brussels, Belgium

[5] Artificial Intelligence Lab, Vrije Universiteit Brussel, Boulevard de la Plaine 2, 1050 Ixelles, Belgium

# Contents

**1 Deriving conditions for viability of safety behaviour** **3**

1.1 When safety behaviour is the preferred collective outcome . . . . . . . . . . . 3

1.2 When safety behaviour is selected by evolution . . . . . . . . . . . . . . . . . . 4

**2 Multiplayer AI race** **10**

2.1 N-player AI Race definition . . . . . . . . . . . . . . . . . . . . . . . . . . . . 10

2.2 Analytical conditions and AIS zones in $N$-team interactions . . . . . . . . . . 12

2.3 Methods: Payoffs over group samplings . . . . . . . . . . . . . . . . . . . . . . 16

**3 Disaster scenarios: personal vs collective risks** **19**

**4 Risk of being found out with longer repercussions** **24**

**5 Average population payoffs** **25**

# 1 Deriving conditions for viability of safety behaviour

## 1.1 When safety behaviour is the preferred collective outcome

We derive analytical condition for which a population of players always following safety precautions has a greater social welfare or average payoff than that of a population of players never following safety precautions, that is, $\Pi_{AS,AS} > \Pi_{AU,AU}$:

$$\frac{B}{2W} + \pi_{11} > (1 - p_r)\left(\frac{sB}{2W} + \pi_{22}\right). \tag{1}$$

Thus,

$$p_r > 1 - \frac{B + 2W\pi_{11}}{sB + 2W\pi_{22}} \tag{2}$$

Following the definitions of different AIS regimes in the main texts, we simplify this condition for the two regimes. First, in the **early AI regime** where $B/W \gg b$, Equation 2 is equivalent to

$$p_r > 1 - \frac{1}{s}. \tag{3}$$

Now, in the **late AIS regime** where $W \to \infty$ (i.e. $B/W \ll b$), Equation 2 is equivalent to:

$$p_r > 1 - \frac{\pi_{11}}{\pi_{22}} = 1 - \frac{b - 2c}{b(1 - p_{fo}^2)}. \tag{4}$$

We can see that the development speed ($s$) is the crucial factor in the early AIS regime while it does not play any role in the late AIS, where for fixed $b$ and $c$, $p_{fo}$ is the only influencing factor.

## 1.2 When safety behaviour is selected by evolution

We now derive conditions for which AS and CS are risk-dominant against AU, which are the case if and only if, respectively,

$$\frac{B}{2W} + \pi_{11} + \pi_{12} > (1 - p_r)\left(\frac{3sB}{2W} + \pi_{21} + \pi_{22}\right). \tag{5}$$

$$\frac{s}{W}\left(\pi_{12} + (\frac{W}{s} - 1)\pi_{22}\right) + \frac{B}{2W} + \pi_{11} > (1 - p_r)\left[\frac{sB}{2W} + \frac{sB}{W} + \frac{s}{W}\left(\pi_{21} + (\frac{W}{s} - 1)\pi_{22}\right) + \pi_{22}\right]. \tag{6}$$

In the **early AI regime** where $B/W \gg b$, both equations are simplified to

$$p_r > 1 - \frac{1}{3s}. \tag{7}$$

On the other hand, in the **late AIS regime** where $W \to \infty$ (i.e. $B/W \ll c$), they are simplified to, respectively

$$\pi_{11} + \pi_{12} > (1 - p_r)(\pi_{21} + \pi_{22}). \tag{8}$$

$$\pi_{11} > (1 - 2p_r)\pi_{22}. \tag{9}$$

which are equivalent to, respectively

$$p_r > \frac{4c(1+s) - b\left(2 + p_{fo}^2 + (-2 + p_{fo}(4 + p_{fo}))s\right)}{b(1 - p_{fo})(1 + p_{fo} + (3 + p_{fo})s)} \tag{10}$$

$$p_r > \frac{1}{2} - \frac{b - 2c}{2b(1 - p_{fo}^2)}. \tag{11}$$

Thus, for safety behaviour to be both selected and the preferred outcome, all the $p_r$ must satisfy all the Eqs (11), (10) and (4).

It is clear to see that the left hand sides of Eqs (11) and (4) are decreasing functions of $p_{fo}$ whenever $b \geq 2c$. We now show that it is also the case for the left hand side of Eq 10. Indeed, its first order derivative by $p_{fo}$ gives

$$-\frac{2(1+s)\left[b\left(4s+p_{fo}^2 s+p_{fo}(3+s)\right)-4c(p_{fo}+s+p_{fo}s)\right]}{b(1-p_{fo})^2(1+p_{fo}+3s+p_{fo}s)^2}$$

which is negative whenever $b \geq 2c$ because

$$\left(4s+p_{fo}^2 s+p_{fo}(3+s)\right)-2(p_{fo}+s+p_{fo}s)=2s+p_{fo}^2 s+p-p_{fo}s>0$$

In short, we have shown that for $b \geq c$, the larger $p_{fo}$ the easier the conditions for the safety behaviour to be both selected and the preferred outcome. Figure S2 validates these observations numerically. Similarly, we also can show that these conditions are harder to achieve the larger $s$ is.

Thus, the hardest conditions are obtained when $p_{fo} = 0$, which is equivalent to

$$p_r > \max\{1-\frac{(b-2c)(s+1)}{2sb}, \frac{4c(s+1)+2b(s-1)}{b(1+3s)}, \frac{c}{b}\}\}. \tag{12}$$

It is easily seen that the right hand side is greater than 1 iff $b < 2c$, i.e. this condition would not be achieved (since $p_r \leq 1$) in that case. Assuming $b \geq 2c$, since $\frac{4c(s+1)+2b(s-1)}{b(1+3s)} > 1-\frac{(b-2c)(s+1)}{2sb} > \frac{c}{b}$, it can be further simplified to

$$p_r > \frac{4c(s+1)+2b(s-1)}{b(1+3s)} \tag{13}$$

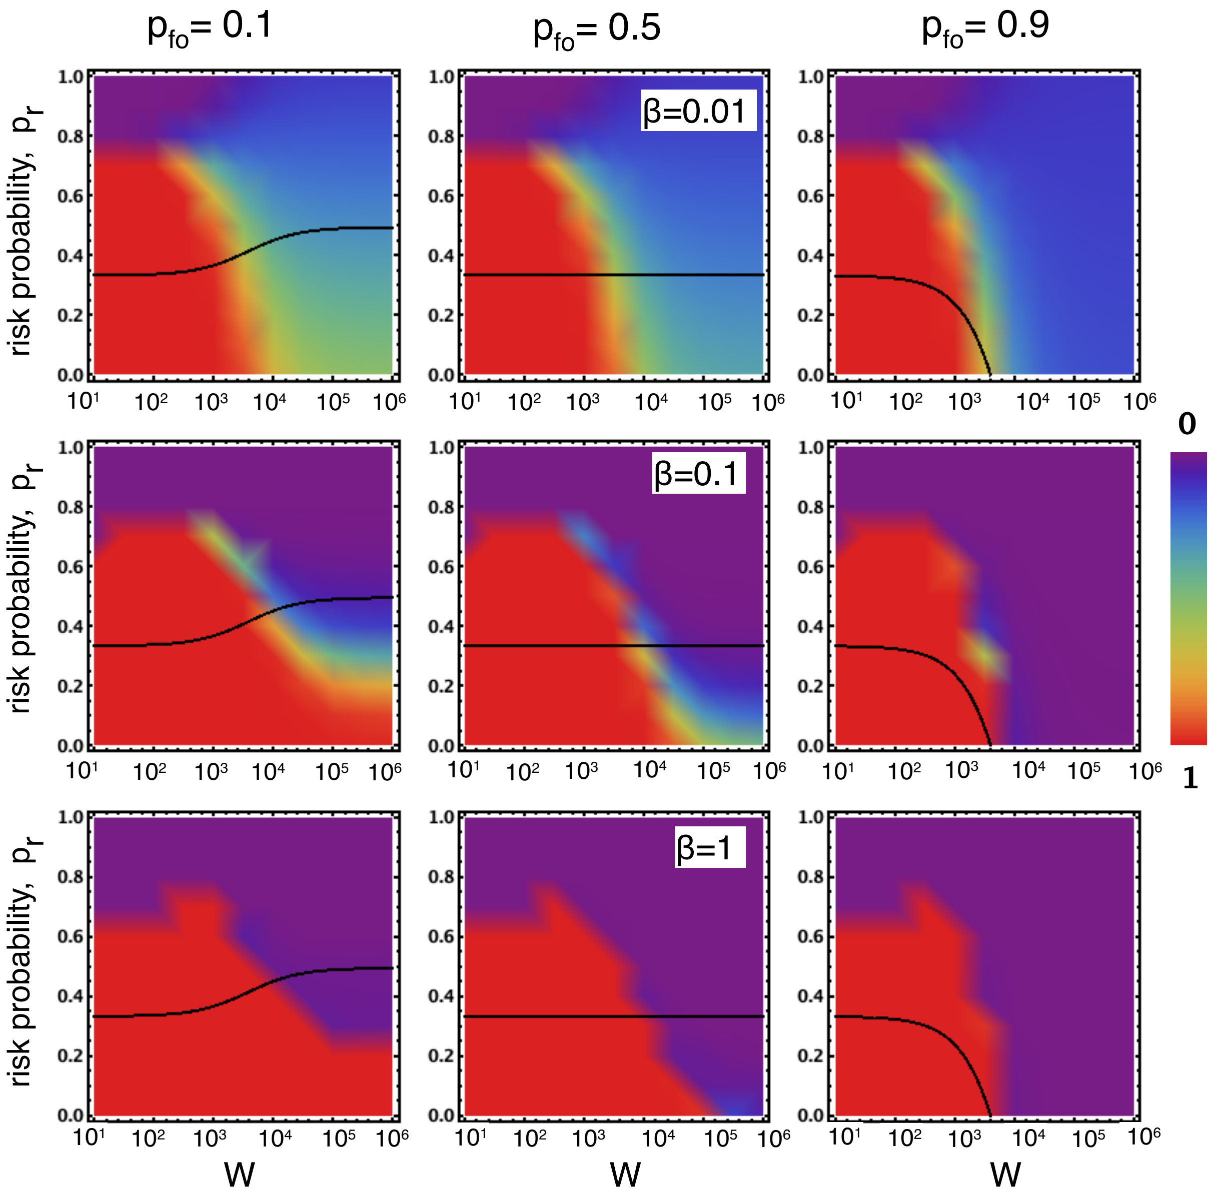


**Figure S1. Across AIS regimes: Frequency of AU** as for varying $p_r$ and different values of $p_{fo}$ and $\beta$: when $W$ is small (early AIS) vs when $W$ is large (late AIS). $\beta = 0.01,\ 0.1,\ 1$ for top, middle and bottom rows, respectively. The *black lines* indicate the threshold of $p_r$ above which SAFE is the preferred collective action and below which UNSAFE is the preferred one (see Equation 2). In general, we observe that AU is dominant for a larger range of $p_r$ in the early than the late regime. Parameters: $c = 1$, $b = 4$, $s = 1.5$, $B = 10000$, $Z = 100$.

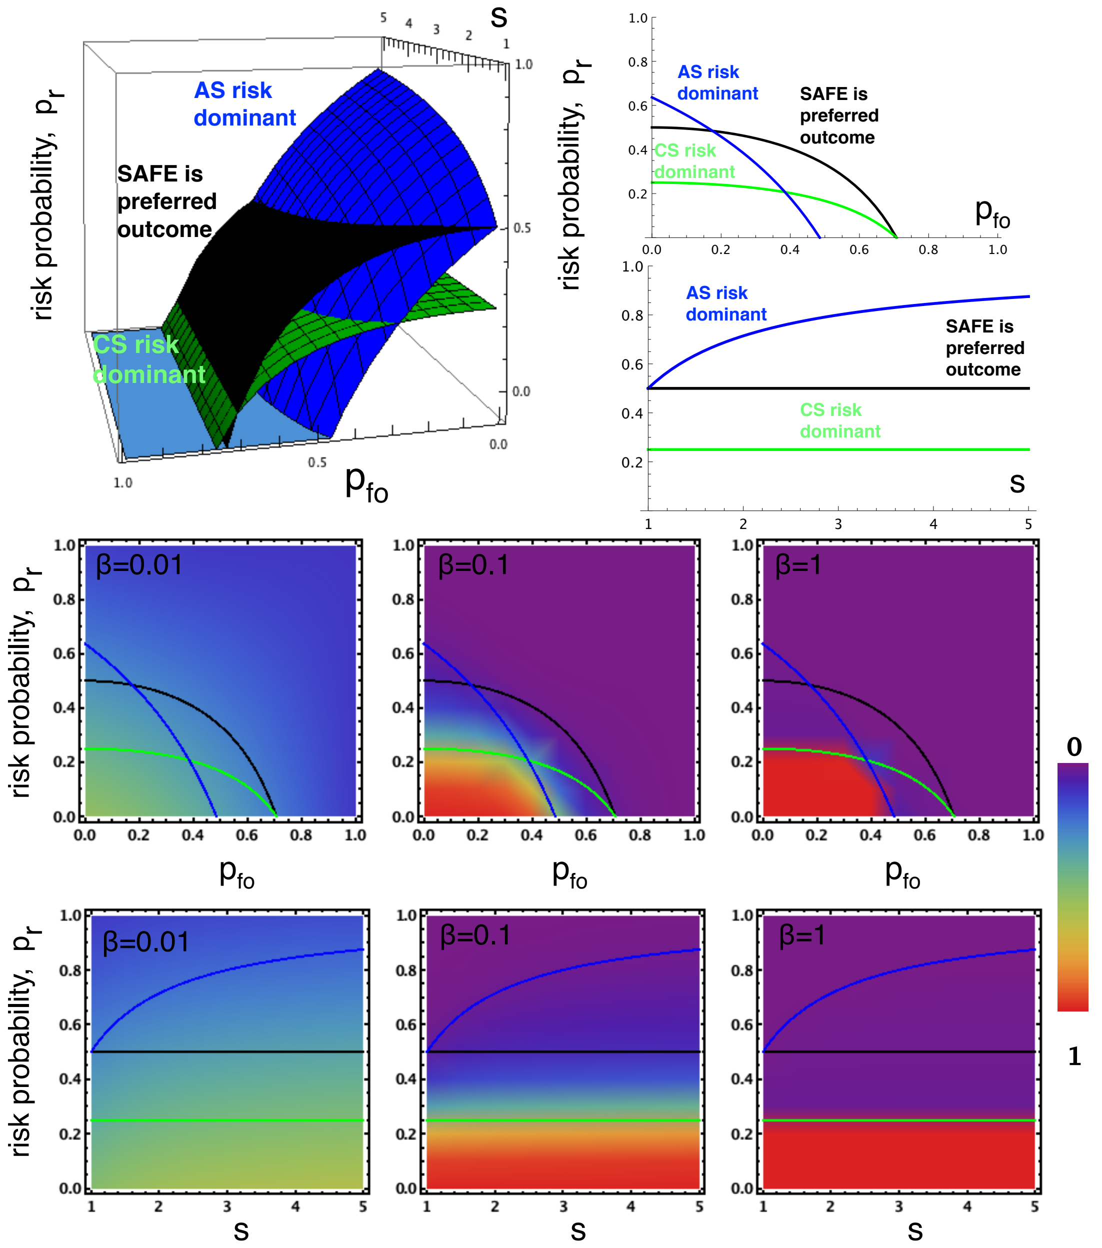


**Figure S2. Late AIS** ($W = 10^6$). The curves/lines indicate the conditions above which safety behavior is the preferred collective outcome (black ones) and when AS and CS are risk-dominant against AU (green and blue ones, respectively). The threshold for AS is greater than than CS when $p_{fo}$ is small, which is reversed when $p_{fo}$ is large **(Top row)**. **(Middle and bottom rows)** Frequency of AU as a function of $p_r$ and $p_{fo}$ (bottom; $s = 1.5$) or $s$ (middle; $p_{fo} = 0$), respectively, for different values of $\beta$. AU has high frequencies in regions below both the blue and green lines, especially for larger $\beta$. Parameters: $c = 1$, $b = 4$, $B = 10000$, $Z = 100$.

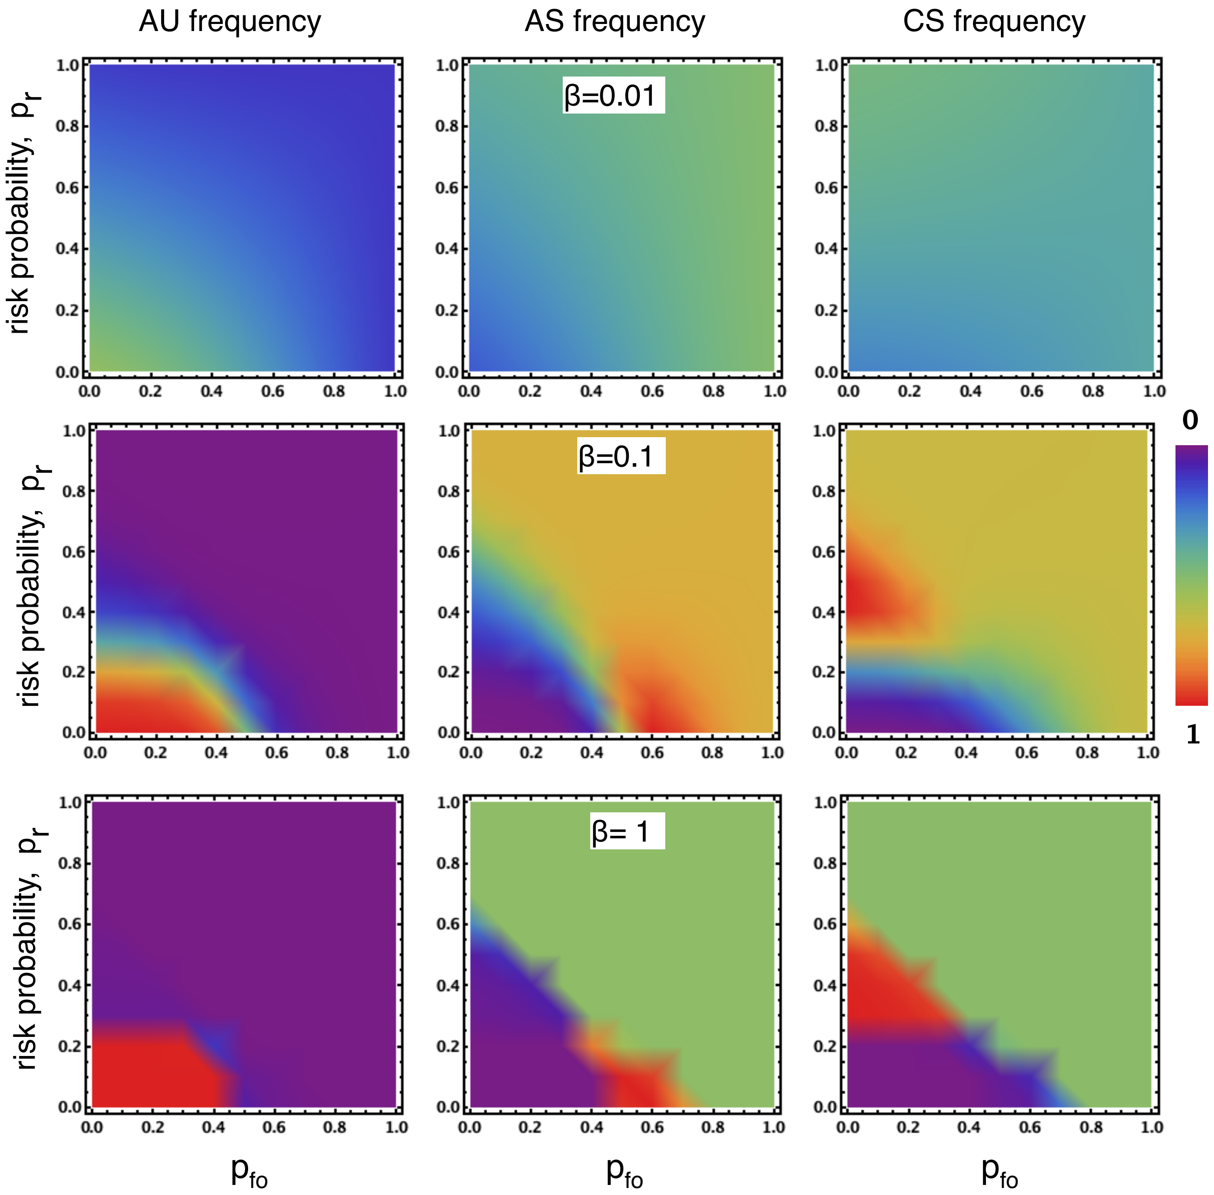


**Figure S3. Late AIS: Frequency of AU, AS and CS** as a function of the probability of unsafe development being found out, $p_{fo}$, and the probability of AI disaster occurring $p_r$, when the number of development steps to reach AIS is very large ($W = 10^6$). $\beta = 0.01,\ 0.1,\ 1$ for top, middle and bottom rows, respectively. AU has a low frequency whenever $p_{fo}$ or $p_r$ are sufficiently high. AS performs best when $p_{fo}$ is large. Parameters: $c = 1$, $b = 4$, $s = 1.5$, $B = 10000$, $Z = 100$.

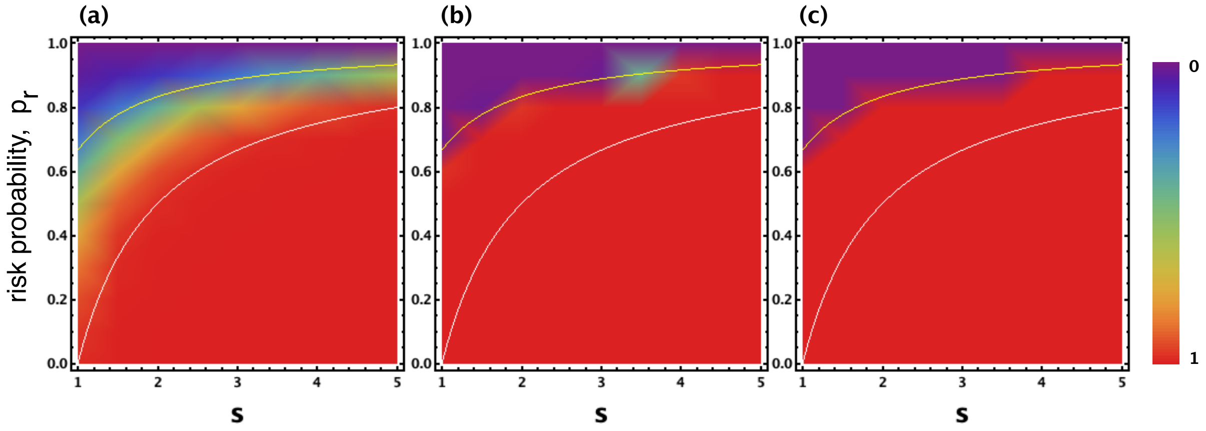


**Figure S4. Early AIS: Frequency of AU in a population of three strategies, AS, AU, and CS**, as a function of the speed gained when ignoring safety, $s$, and the the risk probability $p_r$. In general, we observe that when the risk probability is small, AU is dominant. Also, the larger $B$ and $s$, AU dominates for a larger range. The two solid lines inside the plots indicate the boundaries $p_r \in [1 - 1/(3s), 1 - 1/s]$ where safety development is preferred but non-safety development is preferable (risk-dominant against CS and AS). The observations are valid for varying the selection intensities: $\beta = 0.001,\ 0.01,\ 0.1$ for panels (a), (b) and (c), respectively. Other parameters: $c = 1$, $b = 4$, $W = 100$, $p_{fo} = 0.5$, $B = 10000$, $Z = 100$.

which is the condition for AS to be risk-dominant against AU (see Figure S2 for an example when $s = 1.5$).

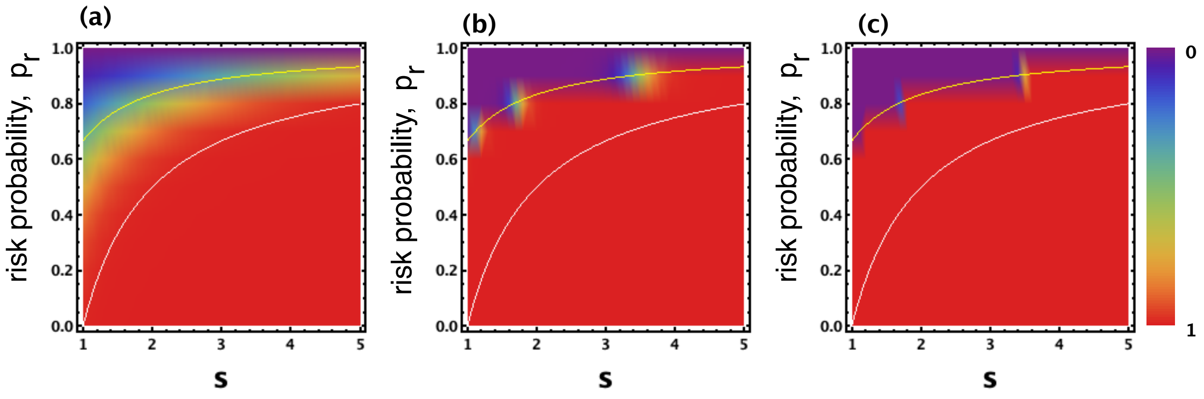


**Figure S5. Early AIS: Frequency of AU in a population of two strategies, AS and AU**, as a function of the speed gained when ignoring safety, $s$, and the the risk probability $p_r$. In general, we observe that when the risk probability is small, AU is dominant. Also, the larger $B$ and $s$, AU dominates for a larger range. The two solid lines inside the plots indicate the boundaries $p_r \in [1 - 1/(3s), 1 - 1/s]$ where safety development is preferred but non-safety development is preferable (risk-dominant against CS and AS). The observations are valid for varying the selection intensities: $\beta = 0.001,\ 0.01,\ 0.1$ for panels (a), (b) and (c), respectively. Other parameters: $c = 1$, $b = 4$, $W = 100$, $p_{fo} = 0.5$, $B = 10000$, $Z = 100$.

# 2 Multiplayer AI race

In this section we describe the N-team model of the AI race, extending the two-team model in the main text. We then describe the Methods used for analysing multi-player games.

## 2.1 N-player AI Race definition

The AI development race is modeled as a repeated $N$-player game, consisting of $W$ development rounds. In each round, the players can collect benefits from their intermediate AI products, depending on whether they choose to play SAFE or UNSAFE. Assuming a fixed benefit, $b$, from the AI market, teams will share this benefit proportionally to their development speed. Moreover, we assume that with some probability $p_{fo}$ those playing UNSAFE might be found out

[1]about their unsafe development and their products won't be used, leading to 0 benefit.

In a group of where $k$ players choosing SAFE and $(N-k)$ choosing UNSAFE, the payoffs for players adopting SAFE and UNSAFE in each round of the race are, respectively

$$\pi(k)_{SAFE} = \begin{cases} -c + (1-p_{fo})\frac{b}{k+s(N-k)} + p_{fo}\frac{b}{k} & \text{if } 1 \leq k < N \\ -c + \frac{b}{N} & \text{if } k = N \end{cases}$$

$$\pi(k)_{UNSAFE} = (1-p_{fo})\frac{sb}{k+s(N-k)} \text{ for } 0 \leq k < N$$

We consider a well-mixed, finite population of size $Z$, where players repeatedly interact with each other in the AI development process, using one of the following three strategies :

- AS (always complies with safety precaution)
- AU (never complies with safety precaution)
- CS (conditionally safe, plays SAFE in the first round; then plays SAFE if everyone in the group plays SAFE in the previous round and plays UNSAFE otherwise)

The average payoffs for the repeated games ($k$ denotes the number of AS or CS when playing with AU)

$$\Pi_{AS,AU}(k) = \begin{cases} \pi(k)_{SAFE} & \text{if } 1 \leq k < N \\ \frac{B}{NW} + \pi(N)_{SAFE} & \text{if } k = N \end{cases}$$

$$\Pi_{AU,AS}(k) = p\left(\frac{sB}{W(N-k)} + \pi(k)_{UNSAFE}\right) \text{for } 0 \leq k < N$$

[1]For simplicity of calculation, we assume that all the UNSAFE players will be found out or not together, e.g. whenever investigation is done then they are found out; otherwise they are not.

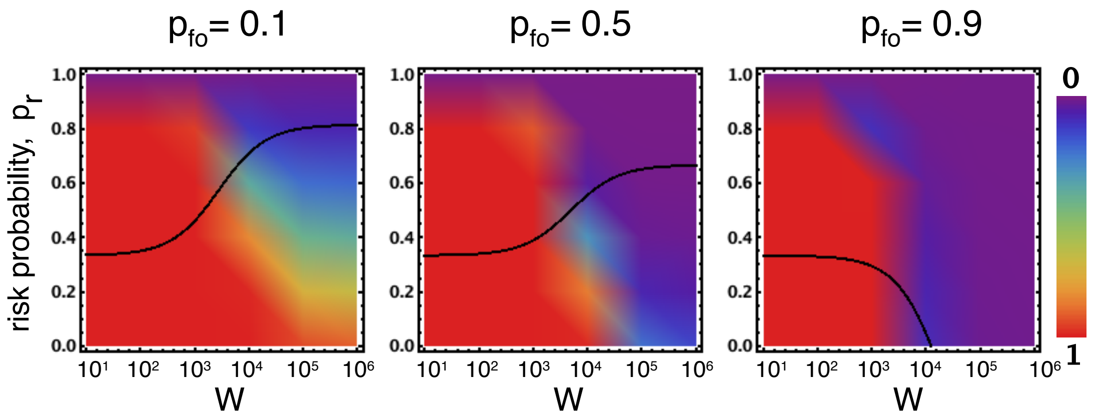


**Figure S6. Different regimes of AIS: early AIS (small $W$) vs late AIS (large $W$), in multi-team game**. Frequency AU in a population of the three strategies AS, AU and CS in co-presence, as a function of $p_r$ and $W$. The black lines indicate the conditions above which SAFE is the preferred collective outcome and below which UNSAFE is (see Equation 14). Other parameters: $c = 1$, $b = 6$, $s = 1.5$, $B = 10000$, $N = 5$, $Z = 100$, $\beta = 0.1$.

$$\Pi_{CS,AU}(k) = \begin{cases} \frac{s}{W}\left(\pi(k)_{SAFE} + (\frac{W}{s} - 1)\pi(0)_{UNSAFE}\right) & \text{if } 1 \leq k < N \\ \frac{B}{NW} + \pi(N)_{SAFE} & \text{if } k = N \end{cases}$$

$$\Pi_{AU,CS}(k) = p\left[\frac{sB}{W(N-k)} + \frac{s}{W}\left(\pi(k)_{UNSAFE} + (\frac{W}{s} - 1)\pi(0)_{UNSAFE}\right)\right] \text{ for } 0 \leq k < N$$

## 54 2.2 Analytical conditions and AIS zones in $N$-team interactions

Condition for $\Pi_{AS,AU}(N) > \Pi_{AU,AS}(0)$, ensuring that a population of players following safety precautions has a greater social welfare or average payoff than that of a population of players never following safety precautions:

$$\frac{B}{NW} + \pi(N)_{SAFE} > (1 - p_r)\left(\frac{sB}{NW} + \pi(0)_{UNSAFE}\right).$$

It can be rewritten as

$$p_r > 1 - \frac{B + W(b - Nc)}{sB + W(1 - p_{fo})b}. \tag{14}$$

In **early AIS** (i.e. $B/W \gg b$), it is equivalent to:

$$p_r > 1 - \frac{1}{s}. \tag{15}$$

which is exactly the same as the condition for pairwise game, and does not depend on the group size $N$.

While in **late AIS** (i.e. $B/W \ll b$), it is equivalent to:

$$p_r > 1 - \frac{b - Nc}{(1 - p_{fo})b}. \tag{16}$$

It can be seen that, for this condition to happen in the late AIS, it is necessary that $b > Nc$. Moreover, the left hand size is an increasing function of $N$ (compare the black lines in Figure S9 for different values of $N$).

Figures S6 shows the results for $N$-player games across different regimes of AIS (i.e. varying $W$). Similar observation is obtained as in the pairwise game in the main text.

**Risk-dominance of AS and CS against AU:** On the other hand, AS and CS are risk-dominant against AU, respectively, iff

$$\sum_{k=0}^{N-1} \pi(k)_{AU,AS} < \sum_{k=1}^{N} \pi(k)_{AS,AU} \tag{17}$$

$$\sum_{k=0}^{N-1} \pi(k)_{AU,CS} < \sum_{k=1}^{N} \pi(k)_{CS,AU} \tag{18}$$

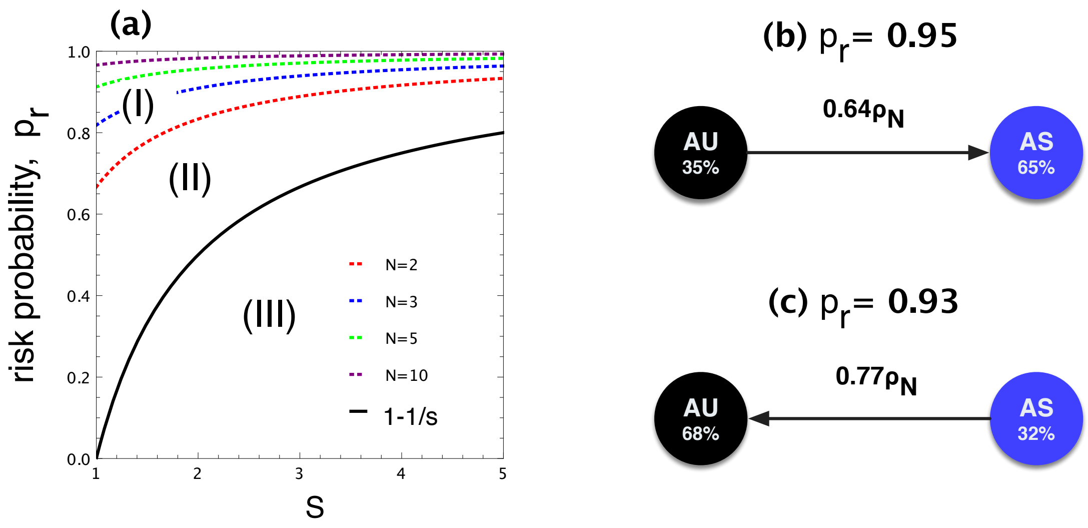


**Figure S7. Early AIS zones in $N$-team interactions.** Dotted lines indicate the condition in Equation 19 for different values of group size $N$. The solid black line indicates the condition in 14. The larger $N$ the larger the region (II) and smaller the region (I). In panels (b), (c): $N = 5$. Other parameters: $c = 1$, $b = 4$, $W = 100$, $s = 1.5$, $p_{fo} = 0.5$, $B = 10000$, $Z = 100$.

In the **early AIS** (i.e. $B/W \gg b$), both conditions are reduced to

$$p_r > 1 - \frac{1}{(NH_N)s}. \tag{19}$$

where $H_N = \sum_{i=1}^{N} 1/i$. Since $H_N > \log N$ we can see that the left hand side of the inequality approaches 1 for increasingly large group size, $N \to \infty$.

Thus, the two boundary conditions in Equations 15 and 19 divide the parameter space $s$-$p_r$ into three regions, see Figure S7a: (**I**) when $p_r > 1 - \frac{1}{(NH_N)s}$: safety development is both the preferred collective outcome and selected by evolution (see Figure S7b for an example: for $s = 1.5$ the condition becomes $p_r > 0.94$); (**II**) when $1 - \frac{1}{(NH_N)s} > p_r > 1 - \frac{1}{s}$: although it is more desirable to ensure safety development as the collective outcome, natural selection/social learning would drive the population to the state where safety precaution is mostly ignored (see Figure S7c for an example: for $s = 1.5$ the condition becomes $0.94 > p_r > 0.33$); (**III**)

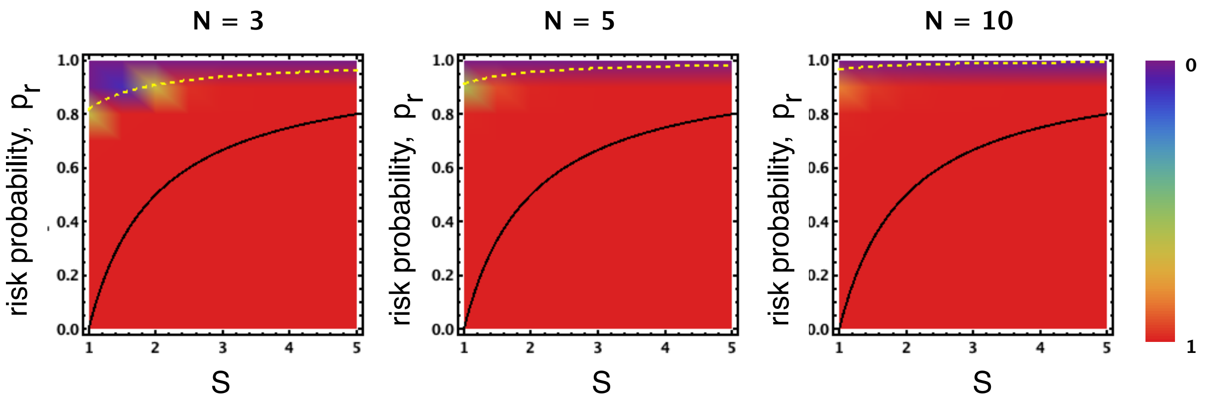


**Figure S8. Early AIS.** Frequency of AU as a function of the speed gained, $s$, and the probability of AI disaster occurring $p_r$, when ignoring safety. Other parameters: $c = 1$, $b = 4$, $W = 100$, $s = 1.5$, $p_{fo} = 0.5$, $B = 10000$, $Z = 100$.

when $p_r < 1 - \frac{1}{s}$, unsafe development is both the preferred collective outcome and selected by evolution. Numerical results (cf. Methods below) in Figure S7 confirm this division of the regions.

We observed that, the larger $s$ is, the greater the threshold for $p_r$. Moreover, a larger group size leads to a larger region (II) – AU is selected for a larger range of the parameter space $s$-$p_r$. The reason is that, the larger the group size, the greater the chance that there is at least one AU player in the group (with other AS/CS players), who would win the development race.

Now, for the **late AIS**, the conditions AS and CS are reduced to

$$p_r > 1 - \frac{\sum_{i=1}^{N} \pi(i)_{SAFE}}{\sum_{i=0}^{N-1} \pi(i)_{UNSAFE}} \tag{20}$$

$$p_r > 1 - \frac{(N-1)\pi(0)_{UNSAFE} + \pi(N)_{SAFE}}{N\pi(0)_{UNSAFE}} = \frac{1}{N}\left(1 - \frac{\pi(N)_{SAFE}}{\pi(0)_{UNSAFE}}\right) \tag{21}$$

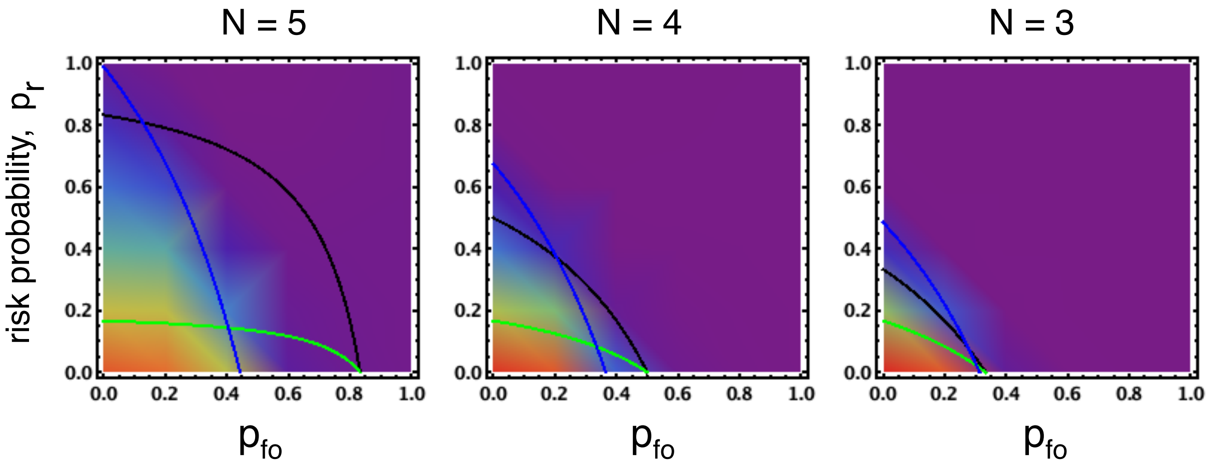


**Figure S9. Late AIS in N-player interactions.** Frequency of AU as a function of $p_{fo}$ and $p_r$ for different competition size $N$. The three lines indicate the conditions as in the main texts (Figure 3). The size of the innovation zone is quite similar for different $N$, but since the larger $N$ the larger the region below the black line (see also analysis), the size of the dilemma zone is increased. Other parameters: $c = 1$, $b = 6$, $s = 1.5$, $W = 10^6$, $B = 10000$, $\beta = 0.1$, $Z = 100$.

## 2.3 Methods: Payoffs over group samplings

In finite populations, the groups engaging in a N-player game are given by multivariate hypergeometric sampling. For transition between two pure states (small mutation), this reduces to sampling (without replacement) from a hypergeometric distribution[2,4]. Namely, in a population of size $Z$ with $x$ individuals of type $i$ and $Z - x$ individuals of type $j$, the probability to select $k$ individuals of type $i$ and $N - k$ individuals of type $j$ in $N$ trials is[2]

$$H(k, N, x, Z) = \frac{\binom{x}{k}\binom{Z-x}{N-k}}{\binom{Z}{N}}.$$

Recall that $\Pi_{ij}(k)$ and $\Pi_{ji}(k)$ (see the section above) denote the payoff of a strategist of type $i$ and $j$, respectively, when the random sampling consists of $k$ players of type $i$ and $N-k$ players of type $j$ (as derived above). Hence, in a population of $x$ $i$-strategists and $(Z - x)$ j-strategists,

the average payoffs to $i$ and $j$ strategists are[2,4]:

$$\begin{aligned} P_{ij}(x) &= \sum_{k=0}^{N-1} H(k, N-1, x-1, Z-1)\, \Pi_{ij}(k+1) \\ &= \sum_{k=0}^{N-1} \frac{\binom{x-1}{k}\binom{Z-x}{N-1-k}}{\binom{Z-1}{N-1}}\, \Pi_{ij}(k+1), \\ P_{ji}(x) &= \sum_{k=0}^{N-1} H(k, N-1, x, Z-1)\, \Pi_{ji}(k) \\ &= \sum_{k=0}^{N-1} \frac{\binom{x}{k}\binom{Z-1-x}{N-1-k}}{\binom{Z-1}{N-1}}\, \Pi_{ji}(k). \end{aligned} \tag{22}$$

Now, the probability to change the number $k$ of agents using strategy $i$ by $\pm 1$ in each time step can be written as

$$T^{\pm}(k) = \frac{Z-k}{Z}\frac{k}{Z}\left[1 + e^{\mp\beta[P_{ij}(k) - P_{ji}(k)]}\right]^{-1}, \tag{23}$$

with $T^{+}$ corresponding to an increase from $k$ tot $k+1$ and $T^{-}$ corresponding to the opposite. As before, $\beta$ expresses the unavoidable noise associated with errors in the imitation process. Fixation probability and stationary distribution are calculated in the same way as in two-player games.

# Risk-dominance condition

An important analytical criteria to determine the evolutionary viability of a given strategy is whether it is risk-dominant with respect to other strategies[1,3]. Namely, one considers which selection direction is more probable: an $i$ mutant fixating in a homogeneous population of agents playing $j$ or a $j$ mutant fixating in a homogeneous population of agents playing $i$. When

the first is more likely than the latter, $i$ is said to be *risk-dominant* against $j$[1], which holds for any intensity of selection and in the limit of large population size $Z$ when

$$\sum_{k=1}^{N} \Pi_{ij}(k) \geq \sum_{k=0}^{N-1} \Pi_{ji}(k). \tag{24}$$

# 3 Disaster scenarios: personal vs collective risks

In the main text we consider that AI risk is personal, i.e. when a disaster occurs due to omitting safety requirements, only UNSAFE players suffer. Here we consider that AI disaster also affects co-players of the interactions. Namely, when a disaster occurs, the UNSAFE players lose their payoffs as before but now their SAFE co-players would lose a fraction of their payoffs, denoted by $\gamma$ ($0 \leq \gamma \leq 1$), with $\gamma = 0$ corresponding to personal risk (as in the main text) and $\gamma = 1$ representing collective risk. So the payoff of AS when playing with AU becomes, in *two-team AI race*: $\pi_{12}(1 - p_r + p_r(1 - \gamma)) = \pi_{12}(1 - p_r\gamma)$. Similarly for CS when playing with AU. Thus, the payoff matrix defining averaged payoffs for the three strategies becomes

$$\Pi = \begin{array}{c} \\ AS \\ AU \\ CS \end{array} \begin{array}{c} \begin{array}{ccc} \quad AS \quad & \quad AU \quad & \quad CS \quad \end{array} \\ \left( \begin{array}{ccc} \frac{B}{2W} + \pi_{11} & (1 - p_r\gamma)\pi_{12} & \frac{B}{2W} + \pi_{11} \\ (1 - p_r)\left(\frac{sB}{W} + \pi_{21}\right) & (1 - p_r)\left(\frac{sB}{2W} + \pi_{22}\right) & (1 - p_r)\left[\frac{sB}{W} + \frac{s}{W}\left(\pi_{21} + (\frac{W}{s} - 1)\pi_{22}\right)\right] \\ \frac{B}{2W} + \pi_{11} & (1 - p_r\gamma)\frac{s}{W}\left(\pi_{12} + (\frac{W}{s} - 1)\pi_{22}\right) & \frac{B}{2W} + \pi_{11} \end{array} \right) \end{array} . \tag{25}$$

Figure S10 shows the results for different values of $\gamma$ across regimes. In the early regime, little difference is observed when moving from completely personal risk ($\gamma = 0$, as in the main text) to mixed risk ($\gamma = 0.5$) and collective risk ($\gamma = 1$). It is also easily seen (similar to the analysis in Section 1 of this SI), the same conditions are obtained in this regime for when AS and CS are risk-dominant against AU as well as when SAFE is the more beneficial collective outcome.

In the late regime, a larger $\gamma$ increases the frequency of AU (The condition under which SAFE is the more beneficial collective outcome, does not depend at all on $\gamma$). They can be

written as follows, respectively

$$\pi_{11} + (1 - p_r\gamma)\pi_{12} > (1 - p_r)(\pi_{21} + \pi_{22}). \tag{26}$$

$$(1 - p_r\gamma)\pi_{22} + \pi_{11} > 2(1 - p_r)\pi_{22}. \tag{27}$$

which are equivalent to, respectively

$$p_r > \frac{\pi_{21} + \pi_{22} - \pi_{11} - \pi_{12}}{\pi_{21} + \pi_{22} - \gamma\pi_{12}} \tag{28}$$

$$p_r > \frac{\pi_{22} - \pi_{11}}{\pi_{22}(2 - \gamma)} = \frac{1}{2 - \gamma} - \frac{\pi_{11}}{\pi_{22}(2 - \gamma)} \tag{29}$$

We can see that the right hand side of the condition of CS is an increasing function of $\gamma$, and when $\gamma = 1$ (shared or collective risk), the condition for CS is the same as for when SAFE is the preferred collective outcome.

Figure S11 shows the frequency of AU in the late regime and the corresponding conditions obtained (see black, blue and green lines). We observe that increasing $\gamma$ enlarges the innovation zones (see the red parts) and reduces the dilemma zone.

Next, similar analysis can be done for the *N-team AI race*. The payoffs of AS and CS when playing with AU is scaled by a factor $(1 - p_r\gamma)$ and all other payoffs remain the same. Similar observations are obtained as in the two-player case. Namely, the same conditions are obtained in the early AIS regime for when AS and CS are risk-dominant against AU as well as when SAFE is the more beneficial collective outcome. For the late AIS, AU is dominant for a larger range for increasing $\gamma$, see Figure S12.

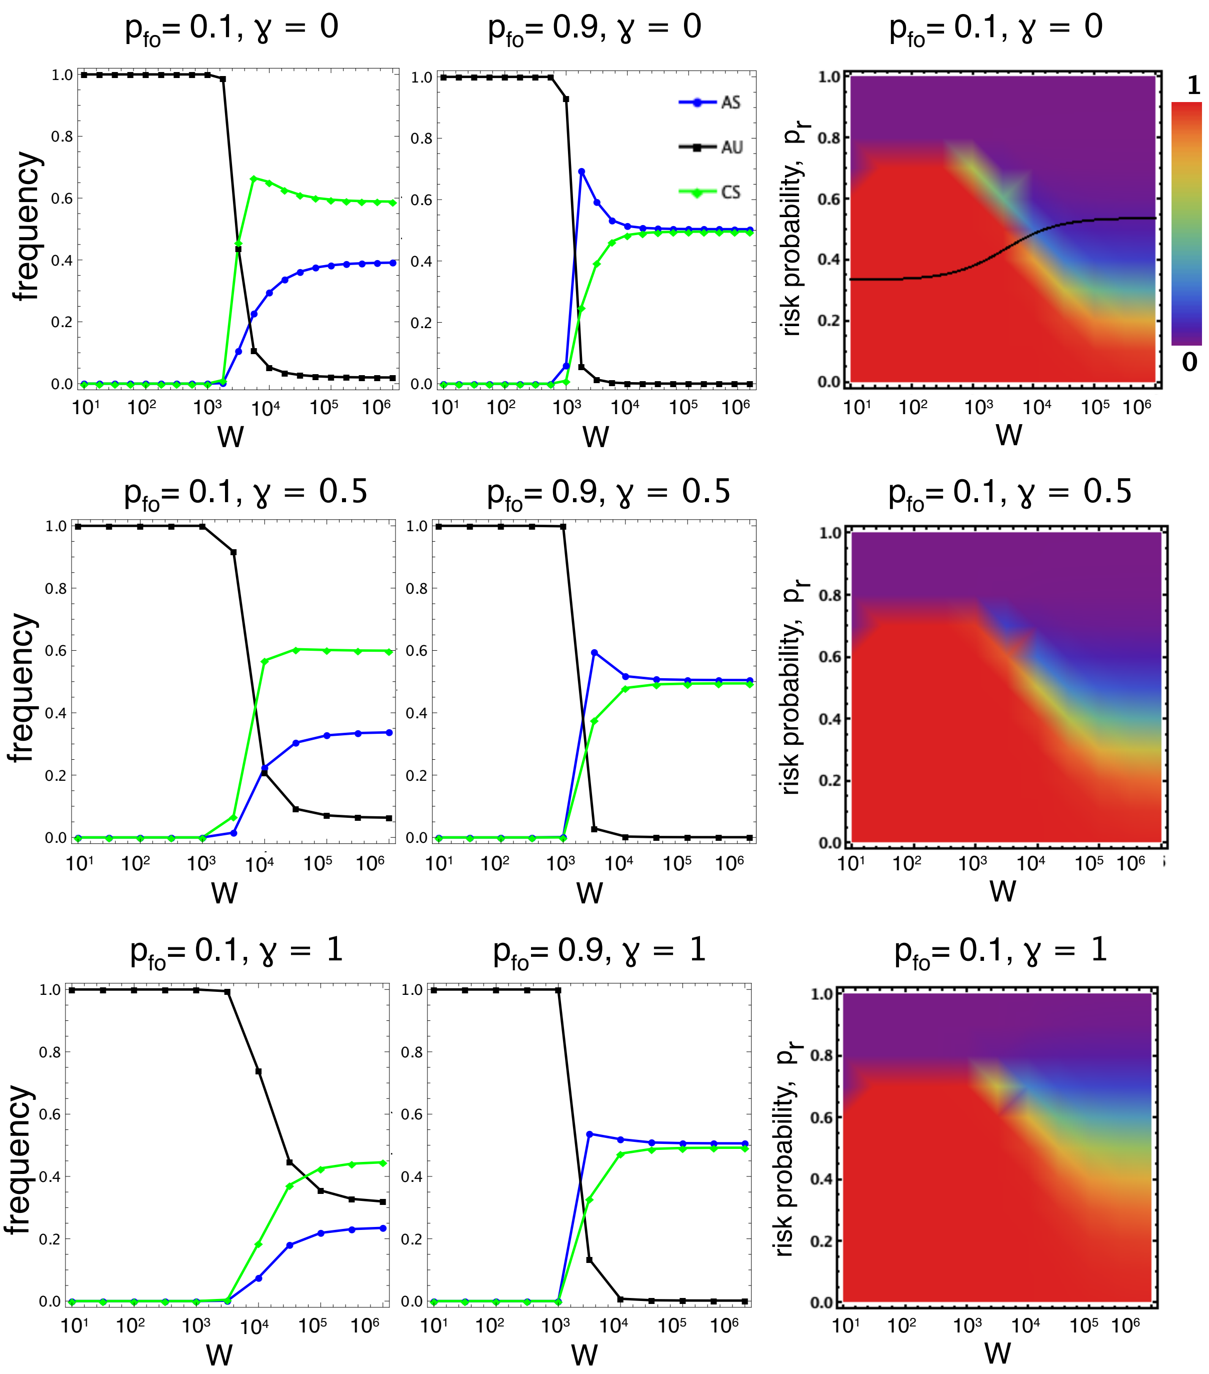


**Figure S10. Different regimes of AIS for different types of risk: when $\gamma = 0$ (top row); $\gamma = 0.5$ (middle row) and $\gamma = 1$ (bottom row)**. Little difference is observed when moving from completely personal risk ($\gamma = 0$) to mixed types of risk ($\gamma = 0.5$) and collective risk ($\gamma = 1$), especially in the early regime. In the late regime, larger $\gamma$ slights increases the frequency of AU. Note that the conditions for which SAFE generates a larger social welfare than UNSAFE behaviour (the black line in the top left panel), does not change with $\gamma$. Parameters: $p_r = 0.6$ (first two columns); $c = 1$, $b = 4$, $B = 10000$, $\beta = 0.1$, $Z = 100$.

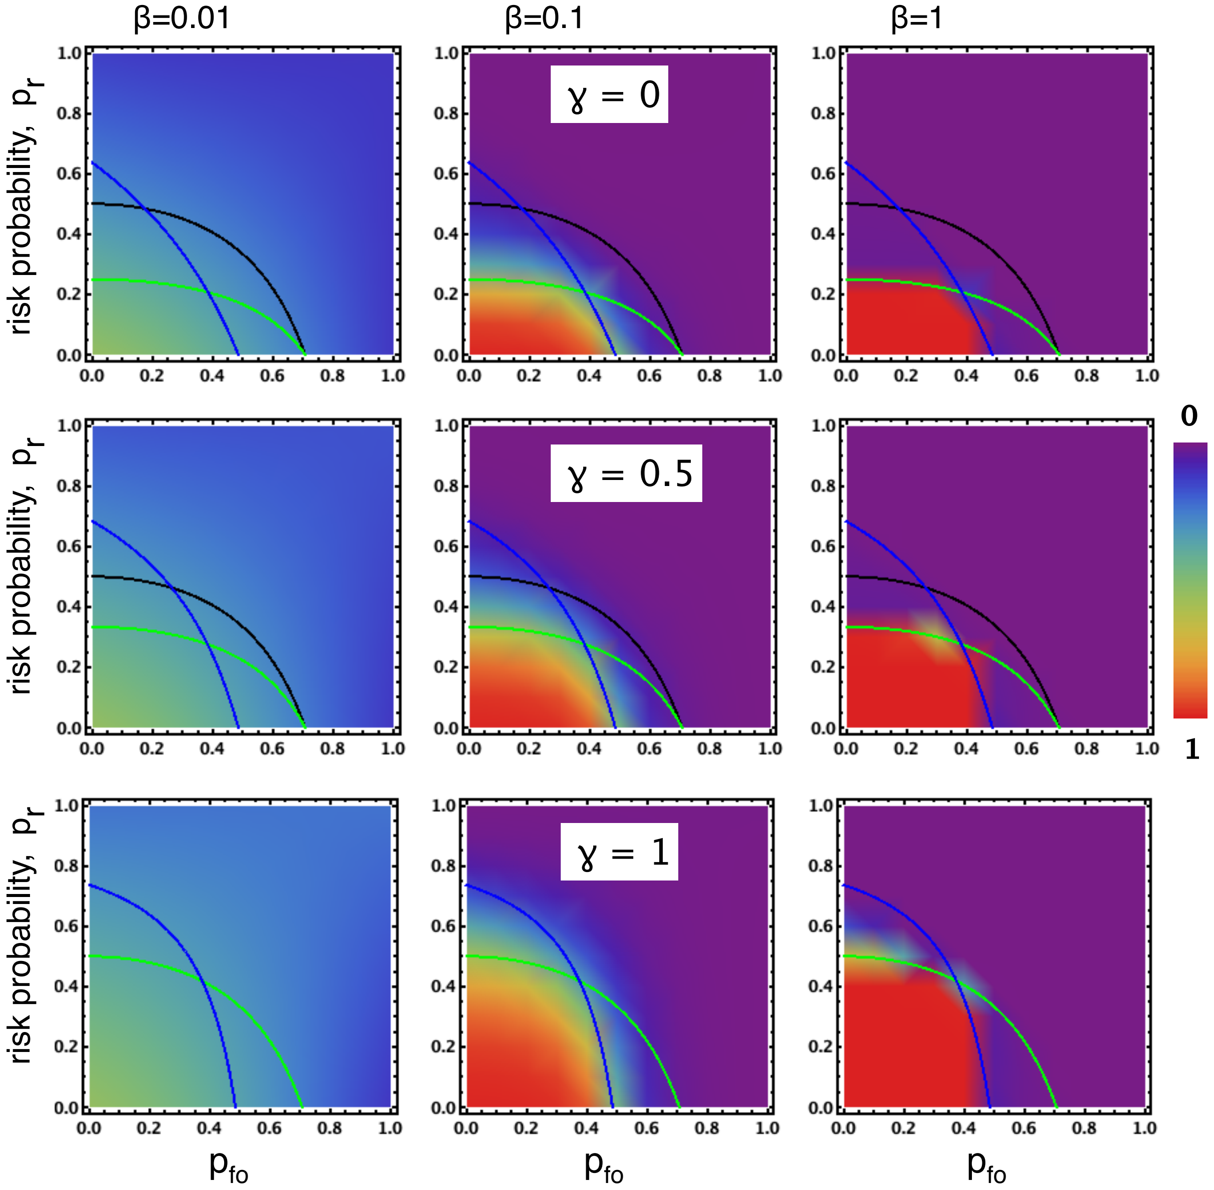


**Figure S11. Late AIS: Frequency of AU when $\gamma = 0$ (top row); $\gamma = 0.5$ (middle row) and $\gamma = 1$ (bottom row).** The three lines (black, blue and green) are the same as in the main text (Figure 3) (in the bottom line the black and green lines are the same). Increasing $\gamma$ enlarges the innovation zones (red parts). Parameters: $c = 1$, $b = 4$, $s = 1.5$, $W = 10^6$, $B = 10000$, $\beta = 0.1$, $Z = 100$.

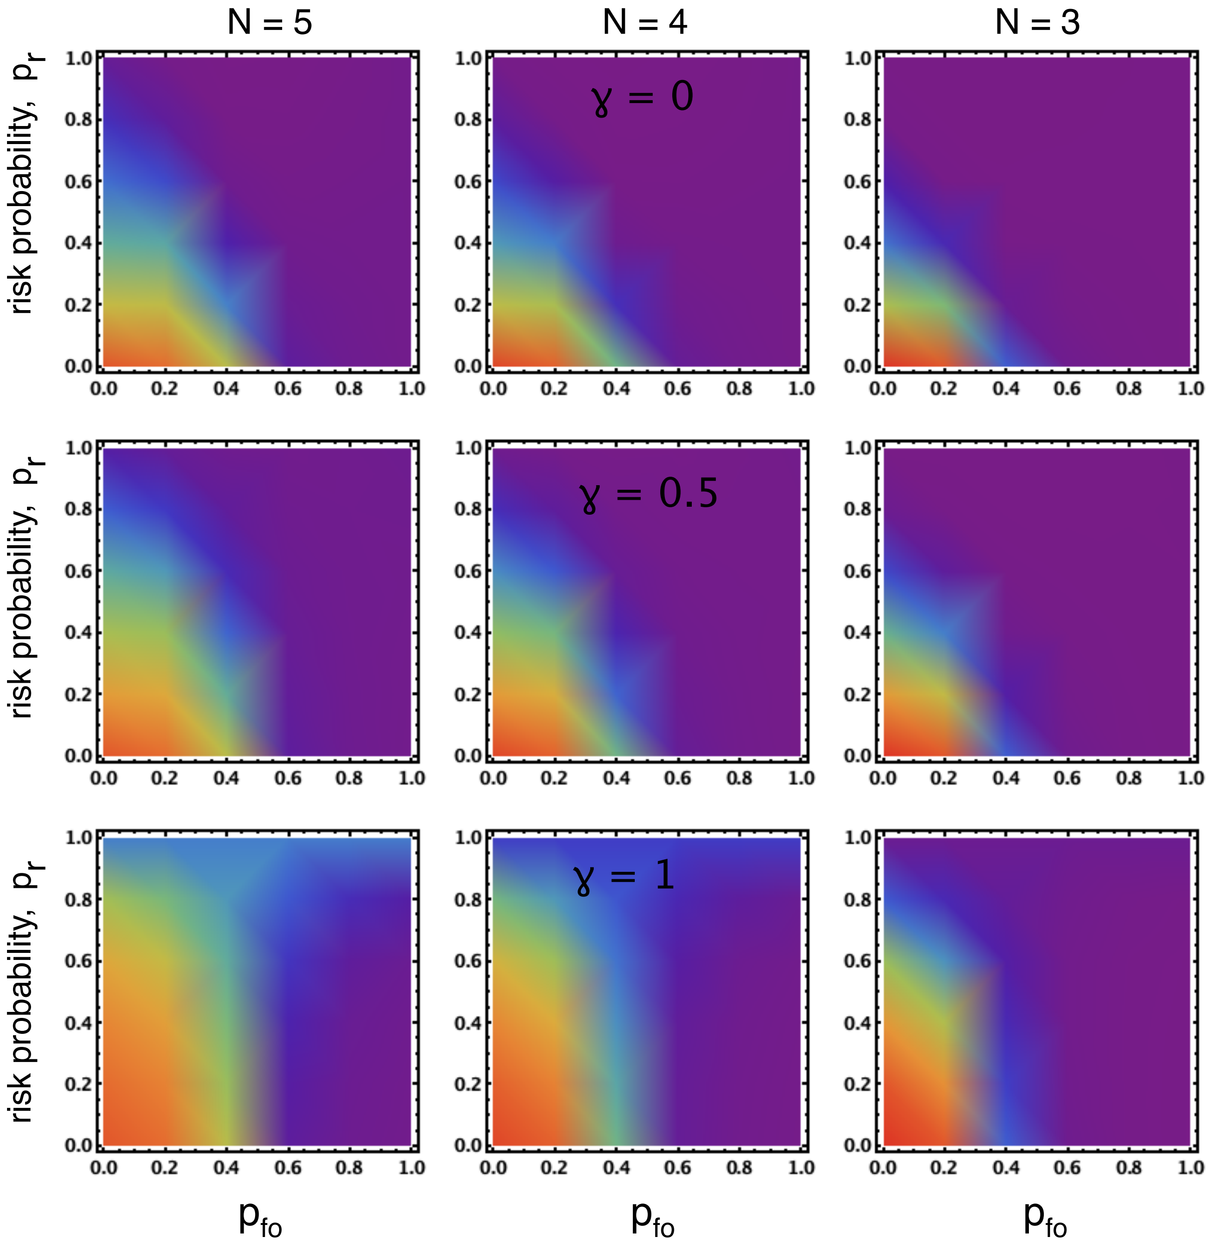


**Figure S12. Late AIS for N-player race: Frequency of AU when** $\gamma = 0$ **(top row);** $\gamma = 0.5$ **(middle row) and** $\gamma = 1$ **(bottom row)**. Increasing $\gamma$ enlarges the innovation zones (red parts). Parameters: $c = 1$, $b = 6$, $s = 1.5$, $W = 10^6$, $B = 10000$, $\beta = 0.1$, $Z = 100$.

# 4 Risk of being found out with longer repercussions

We analyse here the case that the risk of unsafe development being disclosed induces that the found-out unsafe player does not gain her share of $b$ in the subsequent $(u-1)$ (where $1 \leq u \leq W$) rounds. That would clearly reduce the payoffs of AU when interacting with others and increase their payoffs when interacting with AU.

The new payoff matrix defining averaged payoffs for the three strategies reads

$$\Pi = \begin{array}{c} \\ AS \\ AU \\ CS \end{array} \begin{array}{c} \begin{array}{ccc} \quad AS \quad & \quad AU \quad & \quad CS \quad \end{array} \\ \begin{pmatrix} \frac{B}{2W} + \pi_{11} & \tilde{\pi}_{12} & \frac{B}{2W} + \pi_{11} \\ (1-p_r)\left(\frac{sB}{W} + \tilde{\pi}_{21}\right) & (1-p_r)\left(\frac{sB}{2W} + \tilde{\pi}_{22}\right) & (1-p_r)\left[\frac{sB}{W} + \frac{s}{W}\left(\pi_{21} + (\frac{W}{s}-1)\tilde{\pi}_{22}\right)\right] \\ \frac{B}{2W} + \pi_{11} & \frac{s}{W}\left(\pi_{12} + (\frac{W}{s}-1)\tilde{\pi}_{22}\right) & \frac{B}{2W} + \pi_{11} \end{pmatrix} \end{array}. \tag{30}$$

where

$\tilde{\pi}_{21} = \frac{1}{u}\sum_{i=1}^{u}(1-p_{fo})^i \frac{sb}{s+1} = H_u \pi_{21}$,

$\tilde{\pi}_{22} = \frac{1}{u}\sum_{i=1}^{u}(1-p_{fo})^i \frac{(1+p_{fo})b}{2} = H_u \pi_{22}$,

$\tilde{\pi}_{12} = -c + \frac{1}{u}\sum_{i=1}^{u}(1-p_{fo})^{i-1}\left((1-p_{fo})\frac{b}{s+1} + p_{fo}(u+1-i)b\right)$

$\quad = -c + H_u(1-p_{fo})\frac{b}{s+1} + \left(p_{fo}(u+1)H_u + \frac{1-(1-p_{fo})^u}{up_{fo}} - (1-p_{fo})^u\right) b$

where $H_u = \frac{\sum_{i=0}^{u-1}(1-p_{fo})^i}{u} \leq 1$

Thus, exactly the same results are obtained in the early AIS since changing $u$ does not influence the chance of winning the prizes for all strategies.

In the late AIS (i.e. $W \to +\infty$), considering the limit of $u/W \gg 0$ (when found out, a significant portion of the the subsequent rounds are influenced), we have that $H_u \to 0$ and $p_{fo}(u+1)H_u \to 1$ (assuming $p_{fo} > 0$). That has the same effect as having $p_{fo} = 1$ since

$$\tilde{\pi}_{21} \to 0, \quad \tilde{\pi}_{22} \to 0, \quad \tilde{\pi}_{12} \to -c + b$$

# 5 Average population payoffs

In Figure S13 we show the average population payoffs, representing its social welfare. For the early regime (see again Figure 1a in main text), in regions (I) and (III) of the s-$p_r$ space the best possible average payoffs are achieved since SAFE (resp., UNSAFE) population is the one generating a larger payoff than the other and they are also dominating (close to 100% frequency). So no additional mechanism/regulation is required that would change this preferred outcome. In region (II), while SAFE is the outcome with the larger average payoff, since UNSAFE dominates, a significantly lower payoff is obtained. Thus, regulation is crucial to be put in place herein. Note that the highest social welfare is achieved for low $p_r$ and high $s$ (successful innovation), with the dominance of UNSAFE. A misplaced regulation (to achieve SAFE) would destroy this significant social welfare gained through innovation.

In the late AIS regime, see Figure S15, a significant lower social welfare is obtained in this dilemma zone, compared to the one in the unsafe zone, to which regulation can be used to achieve.

# References


1. Chaitanya S. Gokhale and Arne Traulsen. Evolutionary games in the multiverse. *Proc. Natl. Acad. Sci. U.S.A.*, 107(12):5500–5504, March 2010.

2. C. Hauert, A. Traulsen, H. Brandt, M. A. Nowak, and K. Sigmund. Via freedom to coercion: The emergence of costly punishment. *Science*, 316:1905–1907, 2007.

3. Martin A. Nowak. Five rules for the evolution of cooperation. *Science*, 314(5805):1560, 2006.

4. Karl Sigmund. *The Calculus of Selfishness*. Princeton University Press, 2010.

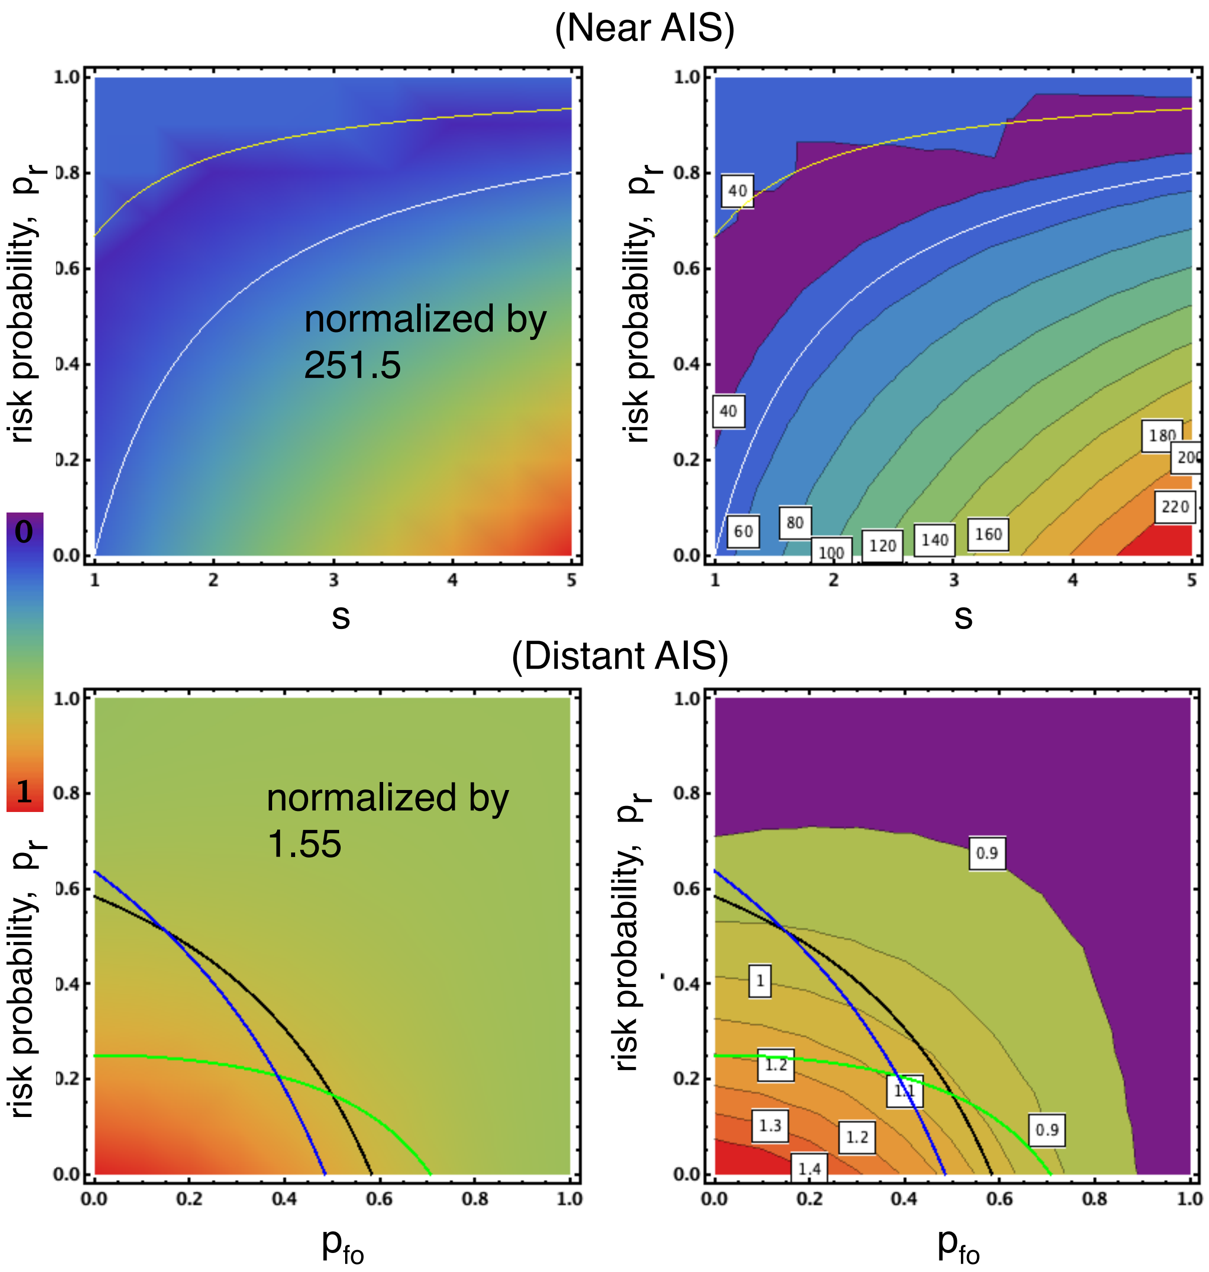


**Figure S13. Average population payoff (social welfare)**. (Top row): early ($p_{fo} = 0.5$); (Bottom row): late regimes ($s = 1.5$). The lines indicate the conditions above which safety behavior is the preferred collective outcome and when AS and CS are risk-dominant against AU. Parameters: $c = 1$, $b = 4$, $B = 10000$, $\beta = 0.01$, $Z = 100$.

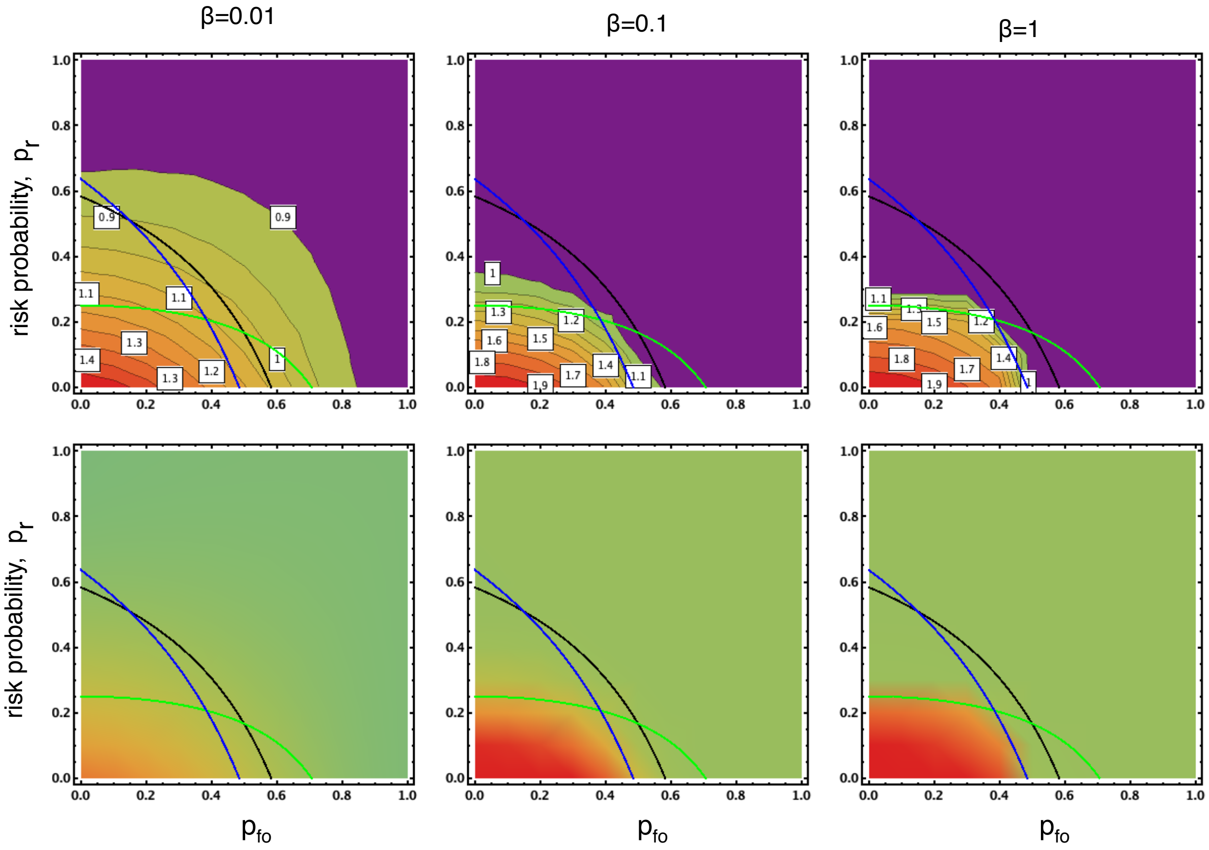


**Figure S14. Late AIS: Average population payoff (social welfare)**. Same parameter settings in in Figure S2. The lines indicate the conditions above which safety behavior is the preferred collective outcome and when AS and CS are risk-dominant against AU. This welfare is significantly lower in the dilemma zone (below black line and above blue and green lines), see also main text discussion. Parameters: $c = 1$, $b = 4$, $B = 10000$, $Z = 100$.

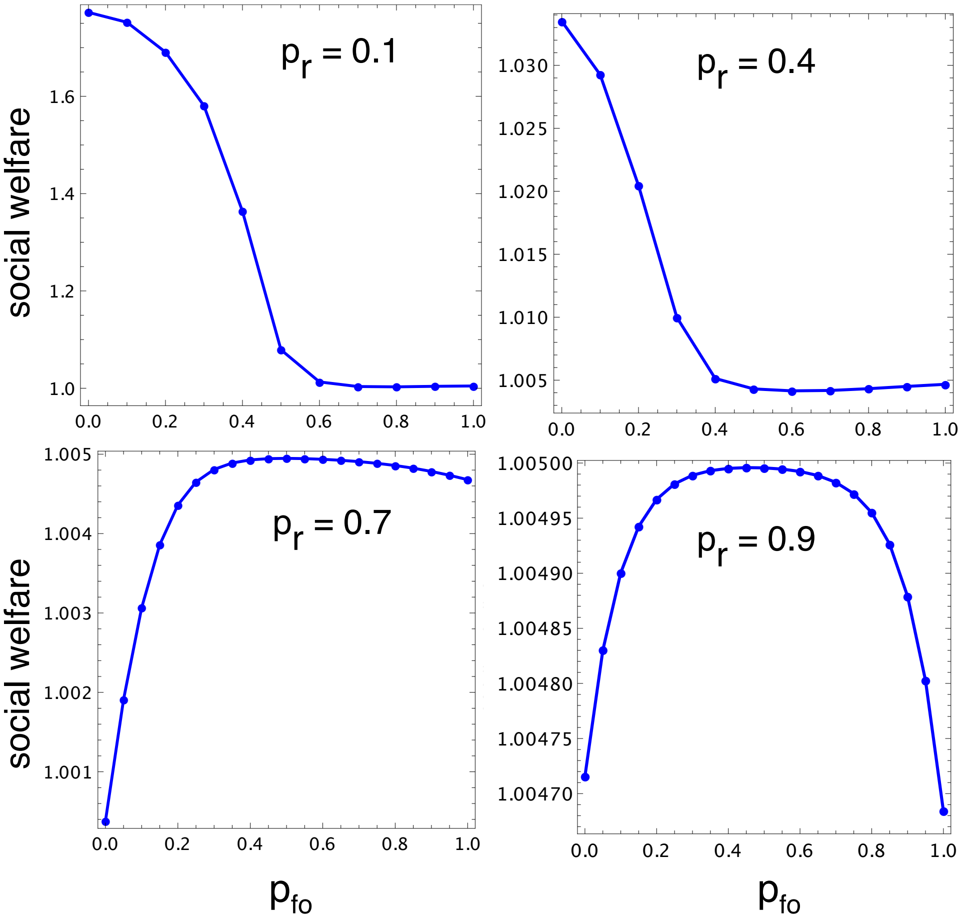


**Figure S15. Late AIS: Average population payoff (social welfare) for varying $p_{fo}$ and different values of $p_r$.** When $p_r$ is small to intermediate, social welfare decreases with $p_{fo}$; while when it is larger, an intermediate $p_{fo}$ leads to the highest social welfare. Parameters: $c = 1$, $b = 4$, $B = 10000$, $s = 1.5$, $\beta = 0.1$, $Z = 100$.
